# Supplementary material for: Precursors to Molecular Slip on Smooth Hydrophobic Surfaces
Source: arXiv:1803.09095 ancillary file (2018-09-05)
Supplement: Supplementary file 1 [file supplemental.pdf]

# Precursors to Molecular Slip on Smooth Hydrophobic Surfaces – Supplemental Information

Justin E. Pye, Clay E. Wood, and Justin C. Burton
*Department of Physics, Emory University, Atlanta, Georgia 30322, USA*

## QCM properties

The experiments utilized a Stanford Research Systems QCM200 + QCM25 system which is designed for liquid immersion. Instead of directly reporting the bandwidth, $\Delta\Gamma$, the QCM200 system reports the equivalent resistance, $R$, of the RLC circuit representing the QCM oscillator, where $R \propto \Delta\Gamma$. We converted the measured resistance in Ohms to the half-bandwidth by varying the temperature of the QCM in the undecane bath around 48°C, and using the fact that $\Delta\Gamma = -\Delta f$ for liquids (Eqns. 1 and 2 in the main text). The result of this calibration is shown in Supplemental Fig. 1.

The quartz wafers were obtained from Inficon and were 330 $\mu$m thick and 2.54 cm in diameter. The exposed electrode material of the crystal was typically gold, although for some experiments they were purchased with an outer layer of $SiO_2$ with thickness 100 nm. The active area, $A_{active} = 37.1$ mm$^2$, of the quartz crystal was measured by placing microliter droplets at various distances from the center of the electrode and observing the response. An approximately Gaussian sensitivity profile was found with a standard deviation of 2.5 mm.

The roughness of the bare QCMs were measured using atomic force microscopy before and after the addition of SAMs. Supplemental Fig. 2 shows a typical image of the surface, and the Fourier transform of the surface height fluctuations. The average RMS value for surface roughness was 1.67 nm, and the lateral length scale for this variation was >100 nm. These length scales result in a negligible contribution to the frequency and bandwidth due to roughness [1], and are not expected to affect slip [2]. In liquids, QCM's emit a very small percentage of their power in the form of longitudinal waves due to gradients in the shear amplitude along the surface [1]. We avoided resonant conditions for emitted longitudinal waves by placing a tilted baffle between the mirror and the chamber window.

The typical amplitude of the crystal oscillation in water, $D_w = 3.3$ nm, was calculated using a 0.5 Volt amplitude across the QCM electrodes from the QCM200 controller [1, 3]. Thus, the shear rate [1] in the water was $\dot{\gamma} = D_w(\rho_w/\eta_w)^{1/2}(2\pi f_0)^{3/2} = 7.7 \times 10^5$ s$^{-1}$. Although this shear rate is larger than encountered in most experiments, low-viscosity liquids such as water are expected to remain Newtonian (i.e. constant viscosity) in this regime [4, 5].

Supplemental TABLE I. Receding ($r$) and advancing ($a$) contact angles (± 2°) for water ($w$) and undecane ($u$) on experimental surfaces in air. The designation (pc) indicates oxygen plasma cleaned, and $\theta^a_{wu}$ indicates a water drop immersed in an undecane bath.

| surface | $\theta^r_w$ | $\theta^a_w$ | $\theta^a_u$ | $\theta^a_{wu}$ |
|---|---|---|---|---|
| $SiO_2$ | 13° | 21° | 0° | 38° |
| $SiO_2$ (pc) | 0° | 0° | 0° | 67° |
| Au | 70° | 95° | 0° | 120° |
| Au (pc) | 0° | 45° | 0° | 115° |
| $Au\text{-}S(CH_2)_{11}CH_3$ | 72° | 90° | 0° | 156° |
| $Au\text{-}S(CH_2)_{11}OH$ | 11° | 50° | 0° | 100° |
| $Au\text{-}S(CH_2)_2(CF_2)_7CF_3$ | 99° | 115° | 0° | 148° |

## Liquid properties

Undecane (> 99% purity) was obtained from TCI America and filtered before each use. De-ionized water was obtained from a Millipore Sigma filtration system. Both liquids were de-gassed using a vacuum pump and flask overnight prior to experiments. A Stanford Research Systems PTC10 temperature controller maintained the undecane bath temperature at 48 ± 0.01°C. Prior to the growth of a water drop on the QCM surface, water was initially added into the corner of the experimental cell to equilibrate with the undecane due to the finite solubility of water in undecane [6] ($1.5 \times 10^{-3}$ mole fraction). This was especially necessary for $SiO_2$ surfaces which displayed reversible, solid-layer adsorption upon the addition of water to the system (Supplemental Fig. 3). The contact area of the drop with the solid surface, $A_{drop}$, was measured by imaging from above. For drops with $\theta^a_{wu} > 90°$, $A_{drop}$ was corrected due to the refraction of the light through the water-undecane surface.

The surface tensions of the water/air, undecane/air, and water/undecane interfaces at 48°C were taken as $\gamma_{wa}$ = 68.0 mN/m [7], $\gamma_{ua}$ = 22.0 mN/m [8], and $\gamma_{wu}$ = 50.0 mN/m [9]. The values for the density and viscosities of water and undecane at 48°C were measured: $\rho_w = 989$ kg/m$^3$, $\eta_w = 5.6 \times 10^{-4}$ Pa.s, $\rho_u = 720$ kg/m$^3$, and $\eta_u$ = $7.8 \times 10^{-4}$ Pa.s.

### Surface preparation

All SAMs were obtained from Sigma Aldrich. The surface of the QCM was initially cleaned by sonication in a Neutrad solution, then rinsed with ethanol and deionized water. The QCM was then plasma cleaned using a custom oxygen plasma oven for 30 s to remove all organic contaminants. For surfaces such as bare gold, this aggressive cleaning procedure was necessary to obtain reproducible results. For SAM surfaces, the QCM was then immersed in an ethanol solution containing the SAM molecules, and left for 24-48 hours. Prior to use in an experiment, the QCM was removed from the solution, rinsed in ethanol, them immediately placed in the QCM25 crystal holder and immersed into the bath of undecane in order to minimize ambient contamination.

### QCM response in a semi-infinite liquid

The QCM is a shear-wave oscillator. When placed in a liquid, the oscillator experiences increased inertia due to the carried mass of the liquid, and increased damping due to the liquid viscosity [1, 10]. The displacement field associated with the elastic shear wave in the quartz crystal with thickness $L$ can be written as

$$\vec{\mathbf{u}}_q = \left(D_{q1}e^{ik_qz} + D_{q2}e^{-ik_qz}\right)e^{-i\omega t}\hat{\mathbf{y}}, \tag{1}$$

where $k_q = \omega\sqrt{\rho_q/\mu_q}$, $\rho_q$ is the density of quartz, and $\mu_q$ is shear modulus of quartz. When transmitted into a semi-infinite liquid of viscosity $\eta_l$ and density $\rho_l$, this shear wave decays exponentially with distance. Assuming $z = 0$ represents the QCM surface, the displacement in the liquid can be written as

$$\vec{\mathbf{u}}_l = D_l e^{-k_lz}e^{ik_lz-i\omega t}\hat{\mathbf{y}}, \tag{2}$$

where $k_l = 1/\delta$, and $\delta = \sqrt{2\eta_l/\rho_l\omega}$ is the viscous penetration depth.

The shear stress in the quartz is given by

$$\tau_{yz} = \mu_q\frac{du_{q,y}}{dz}, \tag{3}$$

and the shear stress in the liquid is

$$\tau_{yz} = \eta_l\dot{\gamma} = \eta_l\frac{d^2u_{l,y}}{dzdt}. \tag{4}$$

We assume that the presence of the liquid contributes a small, complex shift in the frequency from the fundamental resonant frequency, so that $\omega = 2\pi(f_0 + \Delta\tilde{f})$. Thus there are 4 complex unknowns: $D_{q1}$, $D_{q2}$, $D_l$, and $\Delta\tilde{f}$. One of them is an arbitrary amplitude since we are considering linear waves. The 3 equations that determine the 3 remaining unknowns are a continuity of displacement at $z = 0$ (assuming no slip), a continuity of stress at $z = 0$, and a stress free interface at the opposite side of the QCM ($z = -L$). The resulting equations can be solved analytically in the limit $\delta \ll L$, and $|\Delta\tilde{f}| \ll f_0$. The resulting frequency shift is

$$\Delta\tilde{f} = \Delta f_{liq} - i\Delta\Gamma_{liq} = -(1+i)\frac{f_0^{3/2}}{\pi Z_q}\left(\pi\eta_l\rho_l\right)^{1/2}, \tag{5}$$

where $Z_q = \sqrt{\mu_q\rho_q}$ is the acoustic impedance of quartz. Interfacial slip is most easily modeled by altering the displacement continuity boundary condition, but can also be modeled assuming the presence of a thin, viscous layer between the liquid and the quartz (see below).

### QCM response to a thin, viscoelastic film

Deviations from the predicted response of the QCM in liquid (i.e. $\Delta f_{liq}$ and $\Delta\Gamma_{liq}$) can be modeled as a thin, viscoelastic film between the QCM surface and the semi-infinite liquid. For a film of thickness $\Delta z$, the additional shift in frequency and half-bandwidth can be expressed as [1]

$$\Delta f_{film} + i\Delta\Gamma_{film} = -\frac{2f_0^2}{Z_Q}\left(\rho_f - 2\pi i f_0\rho_l\eta_l\tilde{J}\right)\Delta z, \tag{6}$$

where $\tilde{J}$ is the complex shear compliance and the subscripts refer to the film (f) and liquid (l). We have assumed that the QCM is being driven in its fundamental mode. Let us consider two limiting cases. First, for a viscous film where $\mathrm{Re}(\tilde{J}) = 0$ and $\mathrm{Im}(\tilde{J}) = -1/(2\pi f_0\eta_f)$, there is no shift in bandwidth ($\Delta\Gamma_{film} = 0$) and Eqn. 6 reduces to:

$$\Delta f_{film} = \frac{2f_0^2\rho_l}{Z_Q}b, \qquad b = \Delta z\left(\frac{\eta_l}{\eta_f} - \frac{\rho_f}{\rho_l}\right). \tag{7}$$

The apparent slip length $b$ will depend on the relative viscosity and density of the layer. For low-density, depleted layers, which are expected near hydrophobic surfaces, $b$ will to be 10's of nanometers even if $\Delta z$ is small simply due to the fact that $\rho_f < \rho_l$ and $\eta_f < \eta_l$ [11]. However, this continuum model ignores the molecular nature of the surface, and thus ignores transverse variations in the surface potential and does not capture the threshold stress required to initiate slip. Once slip is initiated beyond this critical stress [12], $b$ should increase dramatically, consistent with Eqn. 7.

Second, we can also consider a purely elastic layer, where $\mathrm{Im}(\tilde{J}) = 0$ and $\mathrm{Re}(\tilde{J}) = 1/\mu_f$, where $\mu_f$ is the shear modulus of the layer. In this case Eqn. 6 reduces

to

$$\Delta f_{film} = -\frac{2f_0^2\rho_f}{Z_Q}\Delta z, \tag{8}$$

$$\Delta\Gamma_{film} = \frac{4\pi f_0^3\eta_l\rho_l}{\mu_f Z_Q}\Delta z, \tag{9}$$

so that for soft films ($\mu_f \to 0$), the bandwidth increase significantly, assuming that $\Delta z$ is much less than the wavelength of sound in the film. This is because the amplitude of motion at the liquid-film interface will be larger than the amplitude of motion at the QCM-film interface, and the same amount of energy can be dissipated in the liquid for smaller QCM amplitudes. Despite the continuum nature of the model, it illustrates the role of elastic compliance in the QCM measurements. Prior to the onset of slip, the elastic deformation of near-surface molecules in local potential wells will increase the bandwidth, albeit without the corresponding change in frequency from Eqn. 8. This effect is larger for hydrophobic surfaces with weaker surface interactions.

### Derivation of $\Delta\Gamma_{drop}$

In order to directly relate the excess amplitude of the liquid motion to the increase in bandwidth, we model the QCM as a one-dimensional, driven, damped harmonic oscillator whose dynamics are described by the following equation:

$$\frac{d^2x}{dt^2} + \gamma\frac{dx}{dt} + \omega_0^2 x = \frac{F}{m}\sin(\omega t), \tag{10}$$

where $x$ is the position of the oscillator, $m$ is the mass, $\gamma$ is the damping rate, $\omega_0$ is the natural angular frequency, and $F$ and $\omega$ are the the amplitude and angular frequency of forcing, respectively. We assume that $\gamma \ll \omega_0$ because the QCM has a high quality factor. In this regime, the half-bandwidth at the resonant frequency is given by $\Delta\Gamma = \sqrt{3}\gamma/2$, and the amplitude of motion at the resonant frequency is given by $D = F/(m\gamma\omega_0)$. The total energy dissipated per oscillation cycle is:

$$\begin{aligned}\Delta E =& \int_0^T \gamma m \left(\frac{dx}{dt}\right)^2 dt \\ =& D^2\pi m\gamma\omega_0 \\ =& 2\pi m\omega_0 D^2\Delta\Gamma/\sqrt{3},\end{aligned} \tag{11}$$

where $T = 2\pi/\omega_0$ is the period. Thus the dissipated energy is proportional to the bandwidth and the square of the amplitude of motion. For a QCM immersed in undecane, this implies $\Delta E \propto \Delta\Gamma_{liq}D_u^2$. The growth of the drop will be a small correction to this dissipation, so that to leading order this can be written as $(\Delta\Gamma_{liq} + \Delta\Gamma_{drop})D_u^2$. This can also be written as the sum of the dissipation from the contact areas with undecane and water

$$\begin{aligned}&(\Delta\Gamma_{liq} + \Delta\Gamma_{drop})D_u^2 = \\ &\Delta\Gamma_{liq}D_u^2\frac{A_{active} - A_{drop}}{A_{active}} + \Delta\Gamma_{liq}D_w^2\frac{A_{drop}}{A_{active}}.\end{aligned} \tag{12}$$

We note that $\Delta\Gamma_{liq}$ is the same for both liquids at 48°C because $\eta_w\rho_w = \eta_u\rho_u$. Since the change in amplitude is small, $(D_w - D_s)/D_s \ll 1$ and $(D_u - D_s)/D_s \ll 1$, and to leading order Eqn. 12 reduces to

$$\Delta\Gamma_{drop} = 2\frac{A_{drop}}{A_{active}}\left(\frac{D_w - D_u}{D_s}\right)\Delta\Gamma_{liq}. \tag{13}$$


[1] D. Johannsmann, *The Quartz Crystal Microbalance in Soft Matter Research* (Springer International Publishing, Switzerland, 2015).
[2] N. V. Priezjev and S. M. Troian, J. Fluid Mech. **554**, 25 (2006).
[3] B. Borovsky, B. L. Mason, and J. Krim, J. Appl. Phys. **88**, 4017 (2000).
[4] P. Dontula, C. W. Macosko, and L. E. Scriven, Ind. Eng. Chem. Res. **38**, 1729 (1999).
[5] C. J. Pipe, T. S. Majmudar, and G. H. McKinley, Rheol. Acta **47**, 621 (2008).
[6] D. G. Shaw, A. Maczynski, M. Goral, B. Wisniewska-Goclowska, A. Skrzecz, I. Owczarek, K. Blazej, M.-C. Haulait-Pirson, G. T. Hefter, F. Kapuku, Z. Maczynska, and A. Szafranski, J. Phys. Chem. Ref. Data **35**, 153 (2006).
[7] N. B. Vargaftik, B. N. Volkov, and L. D. Voljak, J. Phys. Chem. Ref. Data **12**, 817 (1983).
[8] A. J. Queimada, I. M. Marrucho, and J. A. P. Coutinho, Fluid Phase Equilibria **4639**, 1 (2001).
[9] S. Zeppieri, J. Rodriguez, and A. L. López de Ramos, J. Chem. Eng. Data **46**, 1086 (2001).
[10] K. K. Kanazawa and J. G. Gordon, Anal. Chem. **57**, 1770 (1985).
[11] D. A. Doshi, E. B. Watkins, J. N. Israelachvili, and J. Majewski, Proc. Nat. Acad. Sci. **102**, 9458 (2005).
[12] A. Martini, H.-Y. Hsu, N. A. Patankar, and S. Lichter, Phys. Rev. Lett. **100**, 206001 (2008).
[13] A. Anderson and W. R. Ashurst, Langmuir **25**, 11549 (2009).

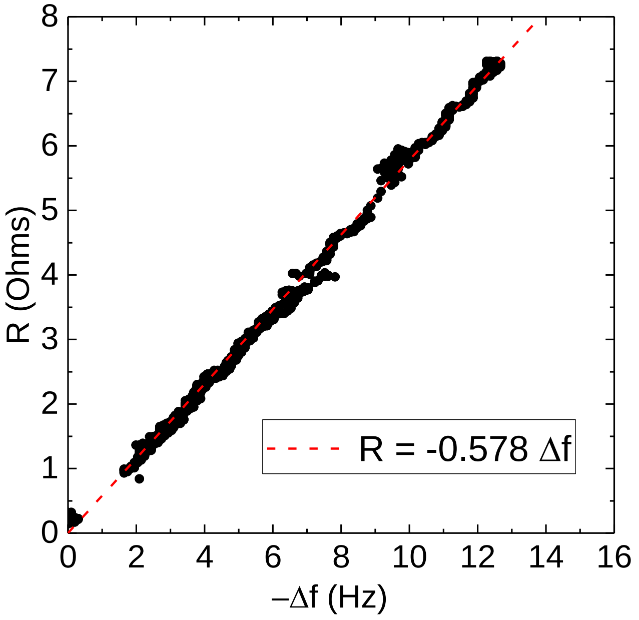


Supplemental FIG. 1. Resistance vs. the change in frequency for a gold-coated QCM immersed in a bath of undecane at 48°C. The data is is the output from the QCM200 system. The variations in $\Delta f$ and $R$ are due to changing the temperature by a few degrees, and was used to compute a conversion factor between $\Delta\Gamma$ and $R$.

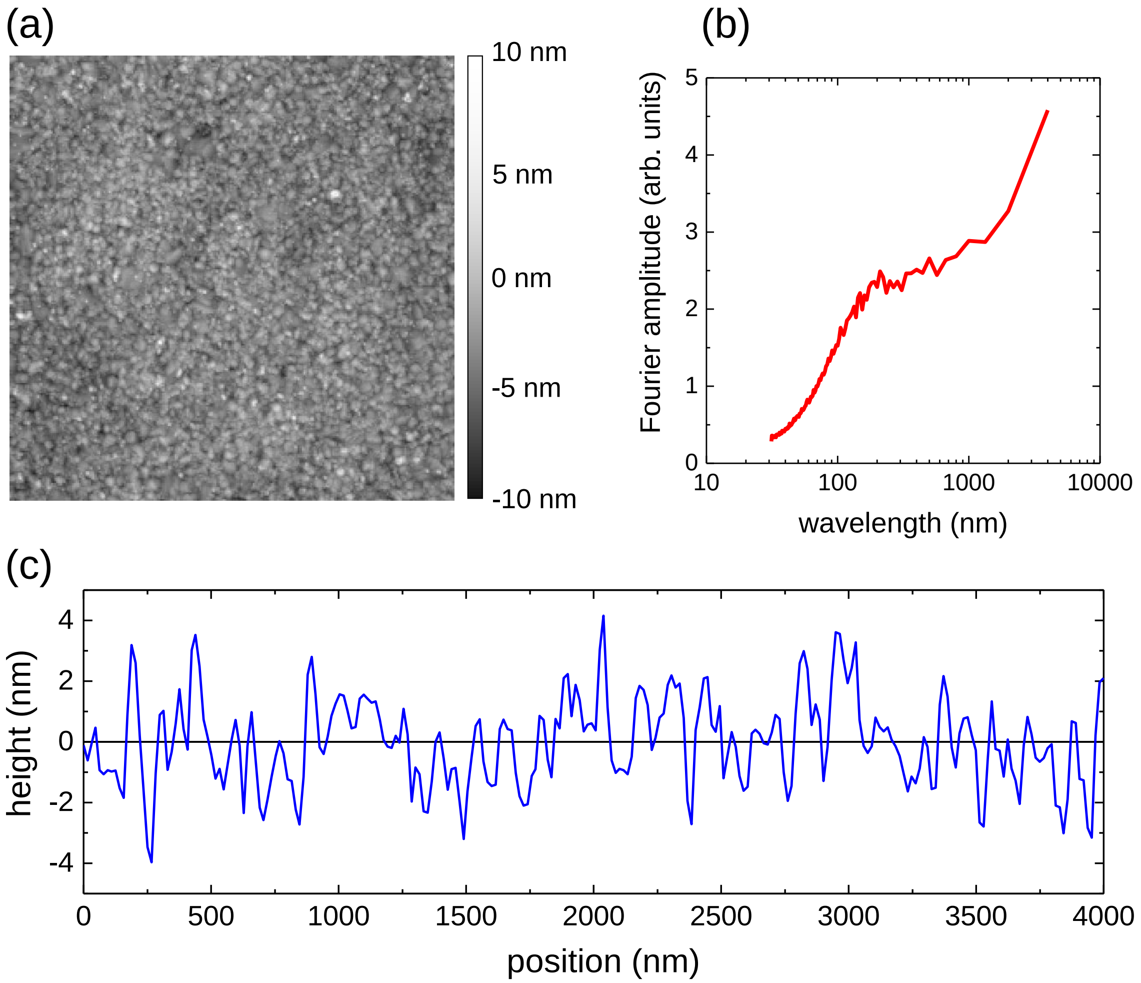


Supplemental FIG. 2. (a) AFM image of a typical Au-S$(CH_2)_{11}CH_3$ SAM surface. The image is dimensions are 4 $\mu$m $\times$ 4 $\mu$m. Maximum and minimum heights are indicated by the color bar. The average RMS amplitude of surface height fluctuations is 1.67 nm. (b) Fourier amplitude vs. wavelength, averaged over horizontal and vertical directions for the surface shown in (a). Most of the variation in height occurs over wavelengths longer than 100 nm, meaning that the surface is locally flat on the molecular scale. (c) Typical line trace showing surface height fluctuations.

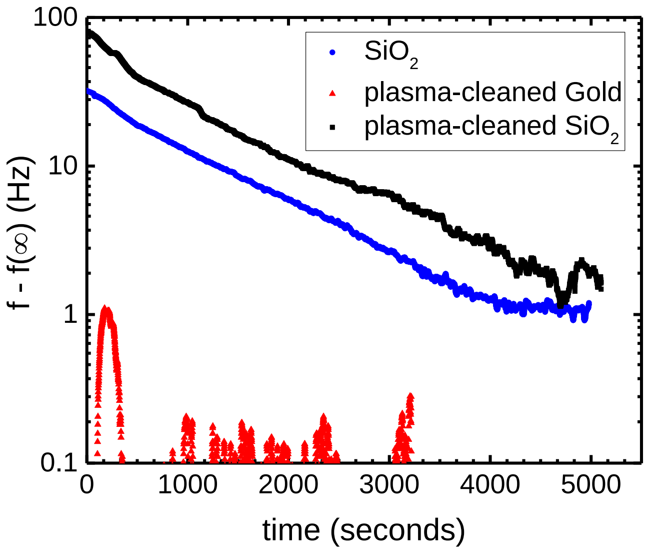


Supplemental FIG. 3. Time dependence of the frequency after the addition of water to the undecane bath for QCMs with $SiO_2$, plasma-cleaned $SiO_2$, and plasma-cleaned gold surfaces. For all surfaces there was no appreciable change in $\Gamma$. For the $SiO_2$ surfaces, the frequency displayed a an exponential relaxation, which we attribute to the adsorption of water molecules at the surface, and thus extra mass carried by the QCM. The effect is larger for plasma-cleaned surfaces, consistent with previous experiments [13]. Assuming bulk values for the density of water, maximum change in frequency after several hours corresponded to 6 nm for $SiO_2$, and 14 nm for the plasma-cleaned $SiO_2$. The effect was completely reversible by allowing the water to evaporate from the undecane bath.

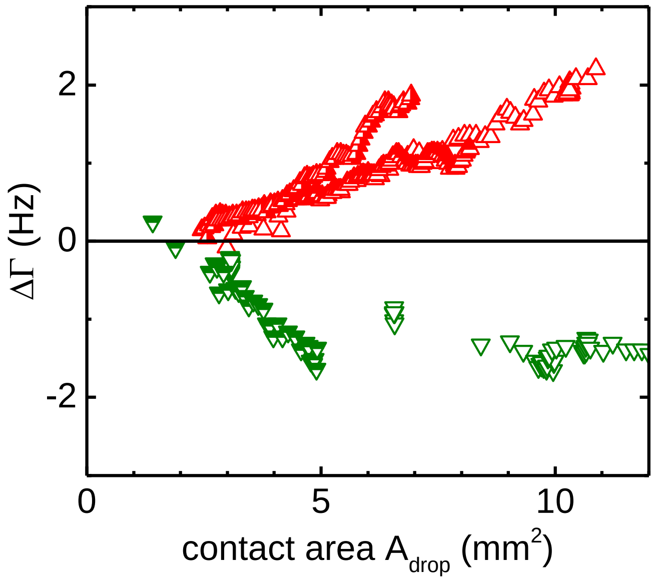


Supplemental FIG. 4. Red up triangles: change in bandwidth during the growth of two separate water drops in an undecane bath on a dodecanethiol-SAM surface ($Au\text{-}S(CH_2)_{11}CH_3$). The advancing contact angle of the drop is $\theta_{wu}^a = 156°$. The same data is shown in Fig. 3a in the main text. Olive down triangles: change in bandwidth during the growth of two separate undecane drops in a water bath. The change in bandwidth reverses sign due to the larger dissipation occurring at the water-solid interface. The advancing contact angle of the drop is $\theta_{uw}^a = 55°$. Gaps in the olive data are due to stick-slip motion of the drop contact line, leading to jumps in the contact area of the drop.
